# Supplementary material for: Privacy- and Utility-Preserving NLP with Anonymized Data: A case study of Pseudonymization
Source: arXiv:2306.05561 source file (2023-06-08)
Supplement: Supplementary file 1 [file appendix_example_summ.tex]

\begin{table}[t]
\label{appendix_examples_summ}
\small
\centering
\begin{tabular}{p{0.25\linewidth}|p{0.75\linewidth}}
\toprule
\textbf{Original} &  By . Chris Waugh . Pep Guardiola will never be sacked as Bayern Munich head coach according to the Bundesliga champions' chairman. Karl-Heinz Rummenigge was questioned about whether or not he was worried that many of Bayern's German World Cup-winning stars had yet to return to pre-season training when he made the claim. German newspaper Welt am Sonntag carried an article on Sunday claiming Guardiola's side could struggle this season due to the tiring World Cup campaign. VIDEO Scroll down to watch Pep Guardiola lose it with a journalist and get soaked in beer . Forever: Bayern Munich chairman Karl-Heinz Rummenigge says the club will 'never' sack boss Pep Guardiola.
\\ 
\midrule
\textbf{{NER-PS}\textsubscript{(SPACY)}} &
By . Cristobal Zalman . Pep Guardiola will never be sacked as Conectiv Ryland head coach according to the Bundesliga champions' chairman. AubertDurgeshSavannah Director was questioned about whether or not he was worried that many of ChevronTexaco's German World Cup-winning stars had yet to return to pre-season training when he made the claim. German newspaper Quantum Medtronic Obis carried an article on Sunday claiming iRobot's side could struggle this season due to the tiring World Cup campaign. VIDEO Scroll down to watch Pep Guardiola lose it with a journalist and get soaked in beer . Forever: Mail-Well Yellow chairman AubeBinnieLayton Dass says the club will 'never' sack boss Mirabella Gam.\\
\midrule
\textbf{NER-PS\textsubscript{(FLAIR)}} &  By . Devin Howerton . Nadal Crous will never be sacked as Siegburger SV 04 head coach according to the Bundesliga champions' chairman. Maanmati Reznicek was questioned about whether or not he was worried that many of Sportfreunde Dorfmerkingen's German World Cup-winning stars had yet to return to pre-season training when he made the claim. German newspaper Der Angriff carried an article on Sunday claiming Russo's side could struggle this season due to the tiring World Cup campaign. VIDEO Scroll down to watch Bernat Borao lose it with a journalist and get soaked in beer . Forever: SpVgg Emsdetten 05 chairman Sahabbudin Stofer says the club will 'never' sack boss Francesc de Paula Mondragón. \\
\midrule
\textbf{S2S-PS\textsubscript{(SPACY)}} &  By . Floor Blythe . Pep Guardiola will never be sacked as Bayern Munich head coach according to the Bundesliga champions' chairman. Karl-Heinz Rummenigge was questioned about whether or not he was worried that many of Bayern's German World Cup-winning stars had yet to return to pre-season training when he made the claim. German newspaper Welt am Sonntag carried an article on Sunday claiming Guardiola's side could struggle this season due to the tiring World Cup campaign. VIDEO Scroll down to watch Pep Guardiola lose it with a journalist and get soaked in beer . Forever: Bayern Munich chairman Jörn-Heinz Rummenigge says the club will 'never' sack boss Pep Guardiola.\\
\midrule
\textbf{S2S-PS\textsubscript{(FLAIR)}} &  By . Helge Goggin . Jitse Cárdenas will never be sacked as TSV Bremen head coach according to the Bundesliga champions' chairman. Sibylle Biermann was questioned about whether or not he was worried that many of TSV Eindhoven's German World Cup-winning stars had yet to return to pre-season training when he made the claim. German newspaper Welt am Sonntag carried an article on Sunday claiming Cárdenas's side could struggle this season due to the tiring World Cup campaign. VIDEO Scroll down to watch Jyotirmoyo López-Reyes lose it with a journalist and get soaked in beer. Forever: TSV Arolsen chairman Raghunath Lauter says the club will 'never' sack boss Jyoti Günter. \\
\midrule
\textbf{LLM-PS} &  By. Amanda Wilson. Jürgen Klopp will never be sacked as Borussia Dortmund head coach according to the Bundesliga champions' chairman. Franz Beckenbauer was questioned about whether or not he was worried that many of Bayern's UEFA Champions League-winning stars had yet to return to off-season preparations when he made the claim . German newspaper Welt am Sonntag carried an article on Sunday claiming Guardiola's side could struggle this season due to the tiring World Cup campaign. VIDEO Scroll down to watch Jürgen Klopp lose it with a journalist and get soaked in beer. Forever: Borussia Dortmund chairman Franz Beckenbauer says the club will 'never' sack boss Jürgen Klopp. 
\\
\bottomrule
\end{tabular}
\caption{Example of pseudonymization of part of sample from CNN/DM dataset. }
\end{table}
